# Supplementary material for: Towards Transferable Multi-modal Perception Representation Learning for Autonomy: NeRF-Supervised Masked AutoEncoder
Source: arXiv:2311.13750 source file (2023-12-06)
Supplement: Supplementary file 1 [file nuscenes_3d_det_fusion_based_appendix.tex]

\begin{table*}[t!]
\small
\resizebox{\textwidth}{!}
	{
	\centering
	\begin{tabular}{l|ccc|ccccc|cc}
          \toprule
         {Method} & {Modality} & {\#Sweep} & {\#ImgSize}   & ATE & ASE & AOE & AVE & AAE   & {{\small{mAP}}} & {{\small{NDS}}} \\ 
         \midrule
          BEVFusion~\cite{liu2022bevfusion}& {LC} &{1} &{$128\times 352$}    &33.3&27.6&59.8&77.6&21.5  & {50.5} &{53.3}\\ 
        + \name & {LC} &{1} &{$128\times 352$}  &33.8&27.4&54.8&73.0&21.4   & \textbf{{{51.5}}} &\textbf{{54.7}}       
         \\         
         \midrule % \midrule
       \textcolor{black}{BEVFusion}~\cite{liu2022bevfusion} & {LC} &{9} &{$256\times 704$}  & &&&& &  {60.8} &{64.1} \\
          + {\name} & {LC} &{9} &{$256\times 704$}   & &&&& & \textbf{{63.0}} &\textbf{{65.5}}  \\ % \midrule
        \bottomrule
	\end{tabular}
       }
     %   \vspace{-1mm}
	\caption{\textbf{3D object detection results for Multi-modal Perception} model (BEVFusion~\cite{liu2022bevfusion}) on \nus{} \cite{Caesar2020nuScenesAM} $val$. The notion of modality: Camera (C), LiDAR (L). \#Sweep denotes the number of Lidar sweeps/scans. \#ImgSize denotes the spatial resolution of input images. The metrics Average Translation Error (ATE), Average Scale Error (ASE), Average Orientation Error (AOE), Average Velocity Error (AVE), and Average Attribute Error (AAE) are supplemented to evaluate the detection ability in a more comprehensive way.
 	}
%\vspace{-4mm}
	\label{tab:nuscene_det_appendix}
\end{table*}
